# Supplementary material for: The mode of host-parasite interaction shapes coevolutionary dynamics and the fate of host cooperation
Source: arXiv:1210.2320 source file (2012-10-08)
Supplement: Supplementary file 1 [file coevcoop_suppl_material.pdf]

# The mode of host-parasite interaction shapes coevolutionary dynamics and the fate of host cooperation

Benjamin J. Z. Quigley, Diana García López, Angus Buckling,
Alan J. McKane, and Sam P. Brown

### SUPPLEMENTARY MATERIAL

## S1 Stochastic methodology

As explained briefly in section II A of the main text, we start the modelling process by specifying the stochastic mechanisms that take place at the microscopic level and result in small discrete changes of the numbers of bacteria and phages. In the simple host-parasite model there are four mechanisms: host birth (bacterial duplication), competition among hosts for finite resources, parasite death (virus degradation) and lysis of a bacterium by a phage. They can be captured by the following reactions:

$$H \xrightarrow{b} 2H\,, \quad 2H \xrightarrow{c} H\,, \quad V \xrightarrow{d} \emptyset\,, \quad H+V \xrightarrow{p} yV\,. \tag{1}$$

Here $b$ is the rate at which each individual host duplicates, i.e. the probability that one host will duplicate during an infinitesimal lapse of time $dt$ is equal to $b\,dt$. If at a given time there are $n_H$ such hosts, the probability that the total number of hosts will increase by one unit during $dt$ due to duplications is $b\,n_H\,dt$. The transition rates $T(\boldsymbol{n'}|\boldsymbol{n})$ at which the composition of the system changes from state $\boldsymbol{n} = (n_V, n_H)$ to state $\boldsymbol{n'} = (n'_V, n'_H)$ can therefore be written as

$$\begin{aligned}
T(n_V, n_H+1|\; n_V, n_H) &= b\; n_H \\
T(n_V, n_H-1|\; n_V, n_H) &= c\; n_H^2/\mathcal{V} \\
T(n_V-1, n_H|\; n_V, n_H) &= d\; n_V \\
T(n_V+y-1, n_H-1|\; n_V, n_H) &= p\; n_H\; n_V/\mathcal{V}
\end{aligned} \tag{2}$$

where $\mathcal{V}$ is the volume of the system.

To describe the change in time of the probability that the system is in state $\boldsymbol{n} = (n_V, n_H)$ at time $t$, $P(\boldsymbol{n}, t)$, one needs to calculate the net effect of in-coming and out-going transitions to and from that state. This is done by a stochastic master equation with the general form

$$\frac{dP(\boldsymbol{n},t)}{dt} = \sum_{\boldsymbol{n'}\neq\boldsymbol{n}} T(\boldsymbol{n}|\boldsymbol{n'})P(\boldsymbol{n'},t) - \sum_{\boldsymbol{n'}\neq\boldsymbol{n}} T(\boldsymbol{n'}|\boldsymbol{n})P(\boldsymbol{n},t)\,. \tag{3}$$

From the master equation we can extract information regarding the evolution of specific quantities of interest. For example, we can derive the macroscopic deterministic ODEs followed by the average concentrations of hosts and parasites ($H$ and $V$) shown in part II A of the main text. For further details of this stochastic population dynamics formalism see McKane & Newman [30].

**Cooperation and coevolution model.** As mentioned in section II C, the benefit from cooperation is captured as an increased birth rate for all hosts, proportional to the fraction of cooperators in the population,

$$b(t) = b_0 + b_1 \frac{n_C(t)}{n_C(t) + n_D(t)}, \tag{4}$$

where $n_C = n_{Ca} + n_{CA}$ and $n_D = n_{Da} + n_{DA}$.

# S2 Host evolution only: details and typical time series

The simplification of the full coevolution and cooperation model (section II C) to recover the model studied in Morgan et al. [29] is as follows. We consider a single type of parasite, $V_a$ (with a zero mutation rate); hosts $(C_a, D_a)$ can however mutate to a resistant type $(C_A, D_A)$. Examples of the typical dynamics can be found in figure S2.

As a measure of the relative fitness of cooperators we use the quantity $\log_{10} v$, where $v$ is computed from the initial and final fractions of cooperators and defectors as

$$v = \frac{x_f^c / x_i^c}{x_f^d / x_i^d} = \frac{x_f^c(1 - x_i^c)}{x_i^c(1 - x_f^c)}. \tag{5}$$

Results are discussed in section III A of the main text.

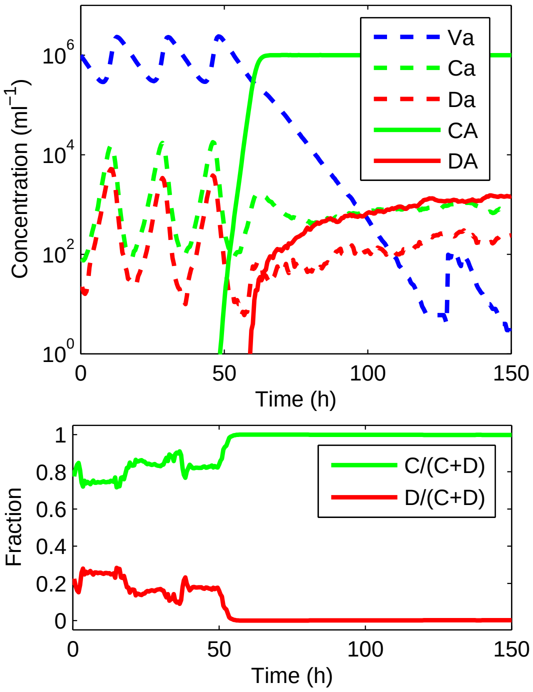


Figure S2: A typical run of the host-evolution-only system (see section III A and S2 text). *Top :* concentration of hosts and parasites as a function of time; *bottom :* fractions of cooperators and defectors in the host population as a function of time. In this example cooperators make up 80% of the initial all-susceptible host population; just before $t = 50$ h a resistant cooperator appears by a random mutation: it quickly takes over, rising to the natural parasite-free carrying capacity of the hosts and causing the virus to start dying out. Here $q = 0$ and the cooperation-defection trait is neutral ($b_1 = 0, w = 0$). Initial conditions are $V_a = 10^6$ ml$^{-1}$, $C_a + D_a = 10^2$ ml$^{-1}$, $V_A = C_A = D_A = 0$; other parameters as in figure 1.

## S3 Full coevolution and cooperation model: time series

The following figures are typical examples of time series of the full model of sections II C and III C of the main text, where hosts have two traits - a non-social one, $a/A$, that determines their resistance to the $a/A$ parasites (see details in main text) and a social trait, $C/D$ (cooperation/defection).

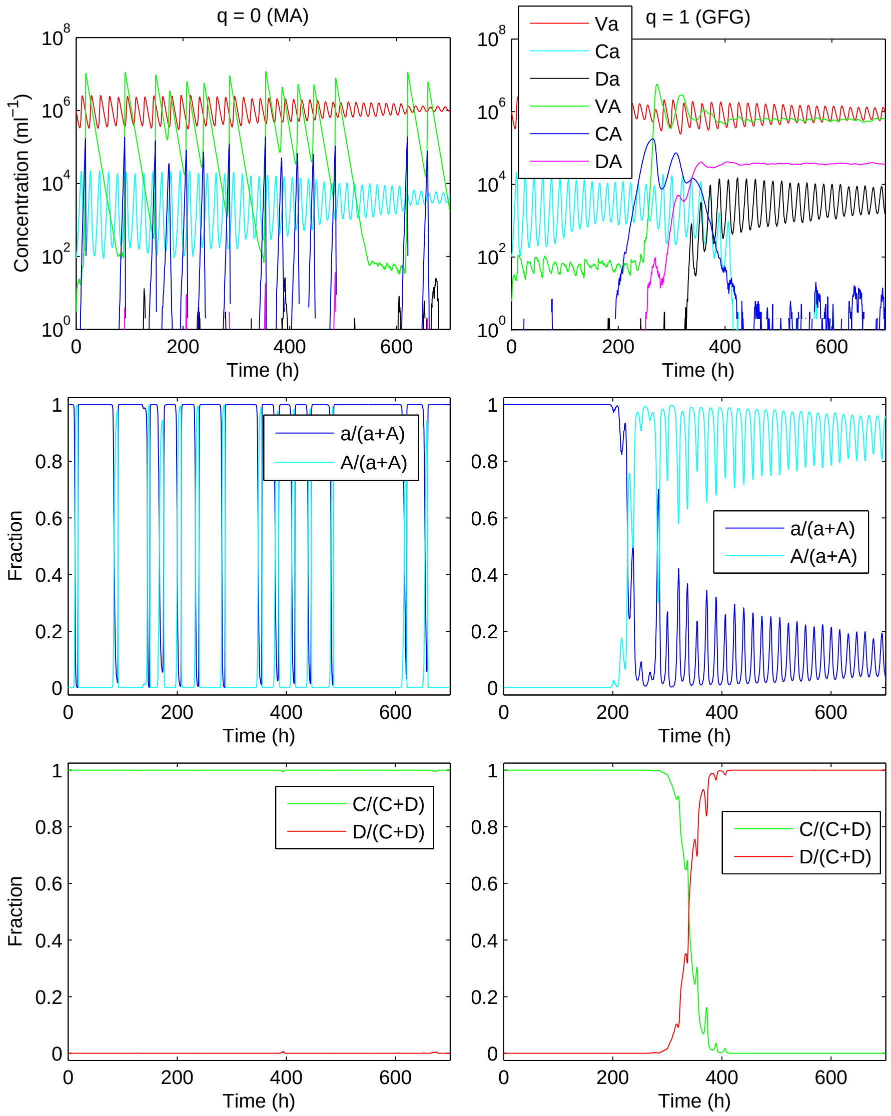


Figure S3: Effect of host-parasite specificity on the maintenance of host cooperation (see sections II C and III C). Examples of stochastic realisations for the two extremes of the MA (*left*, $q = 0$) to GFG (*right*, $q = 1$, $z = 0.9$) continuum. *Top row :* concentration of hosts and parasites as a function of time; *middle :* fractions of $a$ and $A$ alleles in the host population as a function of time; *bottom :* fractions of cooperators and defectors in the host population as a function of time. Parameter values: $p_g = 0.1\,p$, $w = 0.1$; other parameters and initial conditions as in figure 4.

# S4 Host-parasite coevolution model: costs of generalism are required for stability

The following figure corresponds to the model described in sections II B and III B of the main text, where hosts and parasites have a single trait $a/A$ that determines who can infect whom according to the value of the parameter $q$ (see details in section II B). We study how the stability of the host-parasite system depends on the costs of generalism.

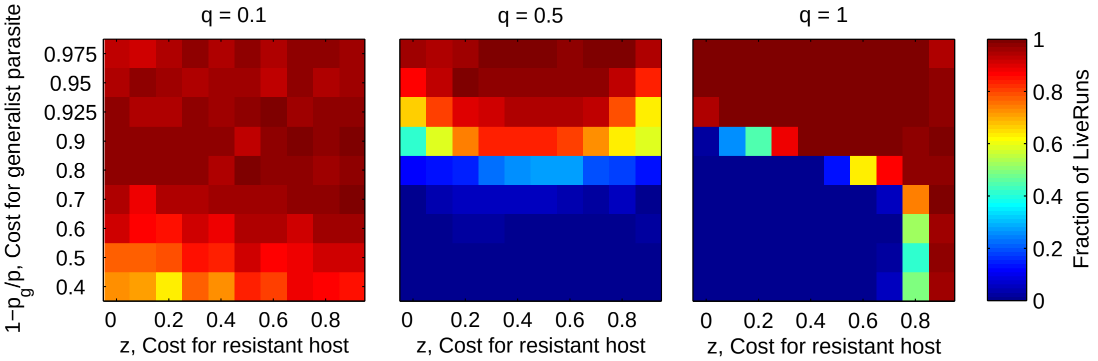


Figure S4: Influence of the costs of generalism on the stability of the host-parasite system in the host-parasite coevolution model (see sections II B and III B). Values plotted are the fraction of runs where hosts and parasites coexist - i.e. where there has not been a global extinction within the 700h observation period. Here $y = 50$ and other parameters and initial conditions are as in figure 3 of the main text. High costs of generalism can be required for stable coexistence of hosts and parasites. With low costs, the generalist parasite overwhelms the host populations and drives them to extinction; its own extinction follows due to the lack of hosts. At higher costs stability is observed.

# S5 Migration scenario: details and figures

What follows are the details of the numerical migration experiments of section III D of the main text. In each realisation we start off with a homogeneous resident host population of type $R$, susceptible to the virus which is also present. This host population is subject to $a/A$ and $C/D$ mutations as usual. At time $t_m$ we add to the system a number of migrant hosts of type $M$, in numbers equal to a fraction $f$ of the *current* population (i.e. at $t_m$) of hosts of the original type. We finally measure the fraction of cooperators at the end of an observation window of length 50h.

We repeat this migration experiment for several pairs of resident $R$ and migrant $M$ types of hosts. We study both the effect of the migrant-to-resident fraction $f$ and of the time of introduction of the migrants $t_m$. See discussion in section III D of the main text and figure S5 below.

Success hardly depends on the relative number of migrants at all, due to the fact that in this host-evolution-only context the resistance trait has no cost associated to it. Mutation opportunities cumulate linearly in time - this is the reason behind the linear dependence with respect to $t_m$ seen in the right graph.

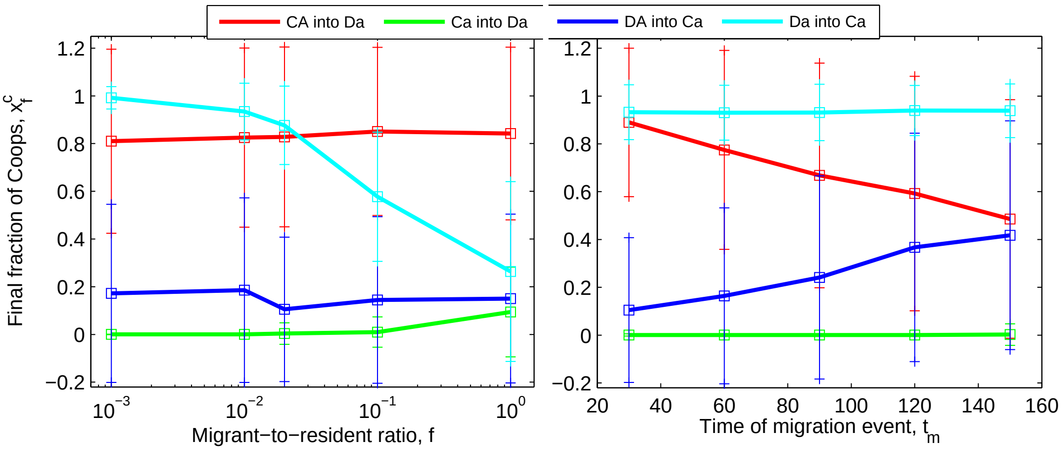


Figure S5: Effect of a single migration event on the fate of an initially homogeneous resident population (see section III D). We plot the final fraction of cooperators as a function of the migrant-to-resident fraction $f$ (the strength of migration), for a fixed time of introduction $t_m = 50$h (*left*), and as a function of the time of arrival $t_m$, for a fixed $f = 0.01$ (*right*). The legend indicates the corresponding migrant and resident types of hosts. Parameter values are $q = 0$, $\mu_V = 0$, $w = 0.05$ h$^{-1}$, $K = 10^6$ ml$^{-1}$, $b_1 = 0.2\, b_0$, $\mu_H = \mu_{cd} = 10^{-6}$ h$^{-1}$, 500 runs per parameter set, rest of parameters as in figure 2. Initial conditions are $V_a = 10^6$ ml$^{-1}$, $V_A = C_A = D_A = 0$ and $\{C_a, D_a\} = \{10^3, 0\}$ or $\{0, 10^3\}$ ml$^{-1}$ depending on their role (resident or migrant – see legend).

# S6 Graphical representation of the models

The specificity relationships between the different types of hosts and parasites configure a network of interactions (similar to a food web) that can be captured in schematic form as shown in the following figure for each of the models studied.

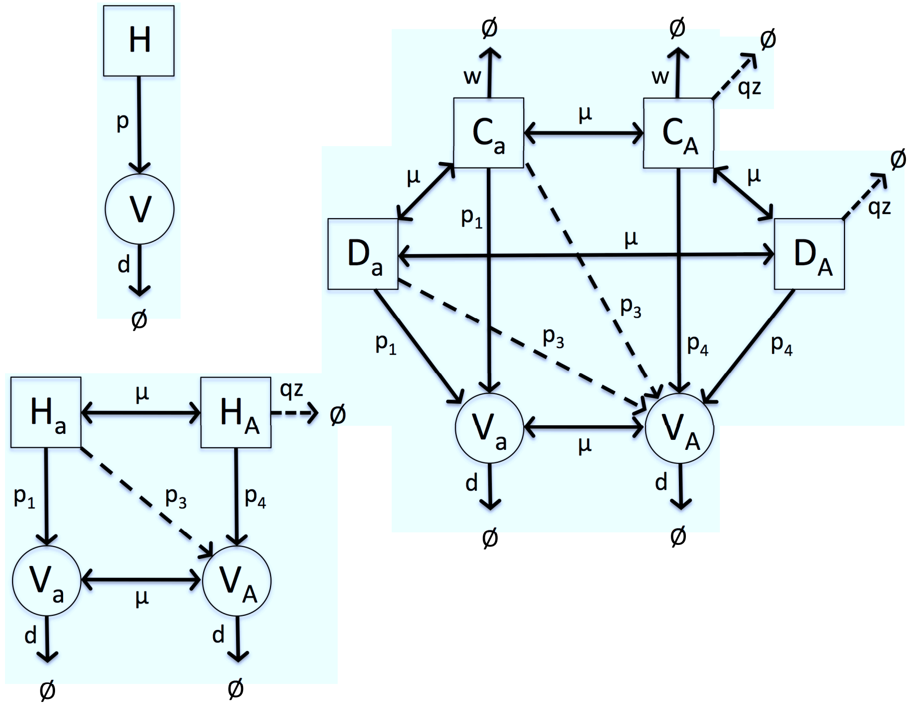


Figure S6a: Schematic representation of the species and (most) mechanisms involved in the simple host-parasite model of section II A (*top left*), the host-parasite coevolution model of section II B (*bottom left*) and the full coevolution and cooperation model of section II C (*right*). Host reproduction and competition are not shown. Dashed lines correspond to links that appear only when $q > 0$. Each arrow representing lysis (predation) stands in fact for a negative feedback loop ($H \rightarrow V$ and $V \dashv H$).

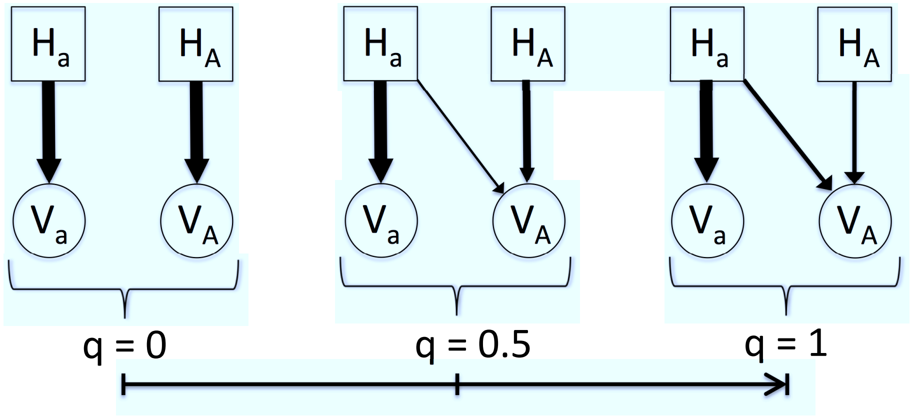


Figure S6b: Schematic representation of the effect of $q$ on the specificity and intensity of the host-parasite interactions (binding affinities, i.e. rates of the lysis reactions) in the coevolution model; see section II B and table 1 of the main text.

# S7 Dependence of the period of host-parasite oscillations on $q$

As was briefly mentioned at the end of section III B, an increase in the MA-to-GFG parameter $q$ implies a decrease of both the binding affinity of $V_A$ to $H_A$ and of the growth rate of $H_A$ (via an increase of the cost of generalist resistance). This in turn seems to cause an increase in the period of the $H_A - V_A$ host-parasite oscillations. In order to elucidate this point, we can apply the same techniques as in McKane & Newman [33] to analytically calculate the dominant period of the host-parasite oscillations in the simple model of section II A. We can thus plot the period $T$ of the oscillations as a function of $q$, as shown in figure S7 below, and find that indeed $T$ increases with $q$.

This sheds light on why in our coevolution and cooperation model the probability of defector takeover grows with $q$. When $q$ is large (GFG), the spacing between the $C_A$ host and $V_A$ parasite peaks is large enough to allow plenty of time for defectors $D_A$ to appear and grow, so that when the $V_A$ hammer falls, they are not completely wiped out (i.e. the density of $D_A$ does suffer a blow but its downward oscillation does not go all the way to extinction). An example of this behaviour can be observed in the top-right panel of figure S3.

Another way of checking this dependence is to modify the current MA model by considering not two equivalent host-parasite pairs but a 'strong' one and a 'weak' one (letting the $H_A - V_A$ pair have a lower binding efficiency and a lower host growth rate, for example by setting $p_1 = p$, $p_2 = p_3 = 0$, $p_4 = p_g$ and imposing a cost on the $H_A$ host); we expect - and find - that cooperation is maintained for much shorter times in such a case.

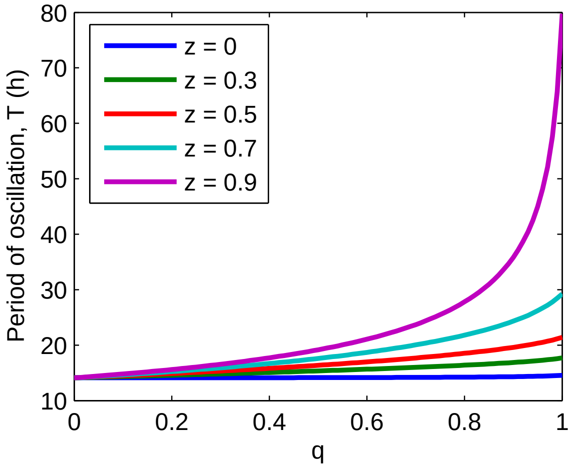


Figure S7: Dominant period of the host-parasite oscillation as a function of $q$, calculated using the technique of McKane & Newman [33], for the simple host-parasite model of section II A. In order to mimic the $H_A - V_A$ pair of the coevolution model, the host growth rate $\tilde{b}$ and the lysis rate $\tilde{p}$ are made to depend on $q$ as follows: $\tilde{b} = b - z\,q$ and $\tilde{p} = q\,p_g + (1-q)\,p$. The dominant frequency of the host-parasite oscillation is given by $T = 2\pi/f$ where $f^2 = \tilde{b}\,\tilde{p}\,d - c\,d^2/(y-1)$. The parameter values used are the same as in figure 3.
